# Supplementary material for: Density Constraints Overcome the Energy-Density Trade-Off in Exchange-Correlation Functionals
Source: arXiv:2610.30022 source file (2026-11-12)
Supplement: Supplementary file 2 [file header.tex]

\usepackage{xcolor}
\usepackage{amsmath,amssymb}
\usepackage{bm}
\allowdisplaybreaks
\renewcommand{\thetable}{S\arabic{table}}
\renewcommand{\thefigure}{S\arabic{figure}}
